# Supplementary material for: Can LLMs Solve longer Math Word Problems Better?
Source: arXiv:2405.14804 source file (2025-02-26)
Supplement: Supplementary file 4 [file results.tex]

\section{Further Results}

\subsection{Training Curves}\label{app: training_curves}

Figure~\ref{fig: training_curve} depicts the {\metrice} and {\metricr} for both LLaMA-2-7B and Mistral-7B throughout 1,200 fine-tuning steps, equivalent to three complete epochs.
Initially, the performance of both models improves rapidly before stabilizing at a later stage. 
This trend underscores the effectiveness of SFT in improving {\property}.

\begin{figure*}
    \centering
    \includegraphics[width=1\linewidth]{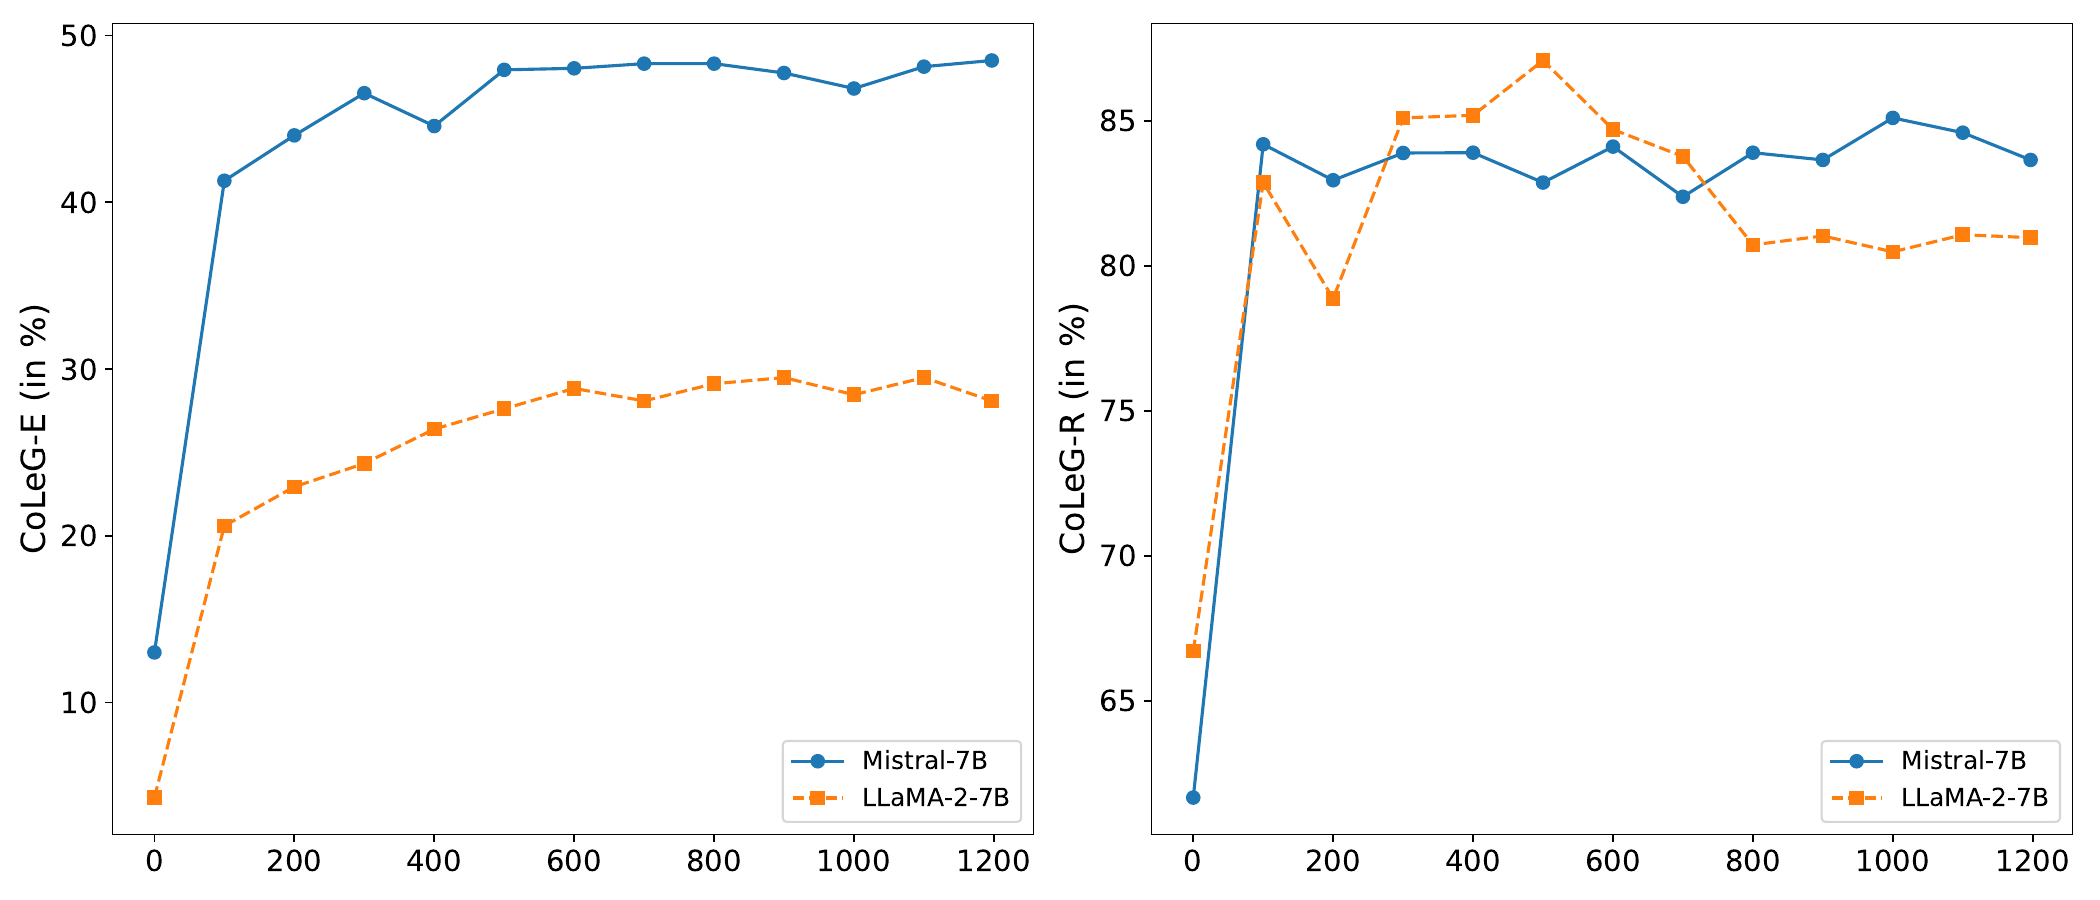}
    \caption{The performance curves of LLaMA-2-7B and Mistral-7B during 1,200 fine-tuning steps. 
    Left: {\metrice};
    Right: {\metricr}.
    The x-axis is the training steps during fine-tuning.}
    \label{fig: training_curve}
\end{figure*}

\subsection{Complete Results of Prompting Methods}\label{app: prompting_rslt}
We have provided some representative results of prompting methods in Table \ref{tab: main_prompt_result} in Section \ref{sec: rslt-prompting}. Here we release complete and detailed prompting results of 7 proprietary LLMs and 4 prompting methods in Table \ref{tabapp: full_prompting_results}. It can be observed that our proposed prompting method achieves notable performance improvement for LLMs with relatively weak proficiency, while relatively subtle enhancement for strong LLMs such as \texttt{GPT-4-turbo} and \texttt{Claude-3-haiku}, which may indicate that these models might find it more challenging to tackle challenges such as extra reasoning requirements brought by long context math problems compared to extracting known conditions.

\subsection{Complete Results of SFT}\label{app: sft_rslt}
Section~\ref{sec: rslt-sft} presents the main results of SFT on {\sftdata}.
The exhaustive results are detailed in Table~\ref{tabapp: sft_full_results}, including 18 LLMs of various scales and base models.
From the results, it is clear that SFT significantly enhances both {\metrice} and {\metricr} in all open-source and math-specific LLMs examined. 
Interestingly, the performance of LLaMA-2 with SFT on the {\sftdata} achieves levels comparable to those of specialized mathematical LLMs. 
It is important to note that our {\sftdata} only consists of approximately 65K entries, whereas MetaMath \citep{metamath2023yu} incorporates around 400K CoT data.

\begin{table*}[ht]
\centering
\footnotesize
\begin{tabular}{ccc|ccccc}
\toprule
\thead{Model} & \thead{CoLeG-E} & \thead{CoLeG-R} & \thead{$\text{Acc}_0$} & \thead{$\text{Acc}_1$} & \thead{$\text{Acc}_2$} & \thead{$\text{Acc}_3$} & \thead{$\text{Acc}_4$} \\
\midrule
\multicolumn{8}{c}{LLaMA-2-7B Models} \\
\midrule
LLaMA-2-7B & 4.31 & 66.71 & 27.37 & 23.93 & 22.83 & 18.97 & 18.26 \\
\rowcolor{gray!25}
 + SFT on D & \makecell{28.09 \\ (+23.78)} & \makecell{80.97 \\ (+14.26)} & \makecell{59.44 \\ (+32.07)} & \makecell{57.57 \\ (+33.64)} & \makecell{50.92 \\ (+28.09)} & \makecell{49.46 \\ (+30.49)} & \makecell{48.13 \\ (+29.87)} \\
 MAmmoTH-7B & 11.52 & 66.09 & 47.46 & 45.02 & 34.91 & 32.67 & 31.37 \\
\rowcolor{gray!25}
 + SFT on D & \makecell{30.15 \\ (+18.63)} & \makecell{80.25 \\ (+14.16)} & \makecell{62.77 \\ (+15.31)} & \makecell{60.00 \\ (+14.98)} & \makecell{54.42 \\ (+19.51)} & \makecell{52.18 \\ (+19.51)} & \makecell{50.37 \\ (+19.00)} \\
 WizardMath-7B & 11.89 & 59.72 & 52.99 & 43.77 & 38.41 & 33.58 & 31.65 \\
\rowcolor{gray!25}
 + SFT on D & \makecell{31.37 \\ (+19.48)} & \makecell{76.77 \\ (+17.05)} & \makecell{63.91 \\ (+10.92)} & \makecell{58.83 \\ (+15.06)} & \makecell{58.09 \\ (+19.68)} & \makecell{52.45 \\ (+18.87)} & \makecell{49.06 \\ (+17.41)} \\
 MetaMath-7B & 31.74 & 74.13 & 66.57 & 62.76 & 54.51 & 51.27 & 49.34 \\
\rowcolor{gray!25}
 + SFT on D & \makecell{38.01 \\ (+6.27)} & \makecell{79.17 \\ (+5.04)} & \makecell{69.07 \\ (+2.50)} & \makecell{65.36 \\ (+2.60)} & \makecell{61.77 \\ (+7.26)} & \makecell{57.62 \\ (+6.35)} & \makecell{54.68 \\ (+5.34)} \\
 \midrule
 \multicolumn{8}{c}{Mistral-7B Models} \\
 \midrule
 Mistral-7B & 13.01 & 61.66 & 50.57 & 45.27 & 39.55 & 37.30 & 31.18 \\
\rowcolor{gray!25}
 + SFT on D & \makecell{48.50 \\ (+35.49)} & \makecell{83.65 \\ (+21.99)} & \makecell{76.12 \\ (+25.55)} & \makecell{74.48 \\ (+29.21)} & \makecell{69.82 \\ (+30.27)} & \makecell{66.70 \\ (+29.40)} & \makecell{63.67 \\ (+32.49)} \\
 WizardMath-Mistral-7B & 50.94 & 79.13 & 82.71 & 76.90 & 70.78 & 68.78 & 65.45 \\
\rowcolor{gray!25}
 + SFT on D & \makecell{52.81 \\ (+1.87)} & \makecell{82.72 \\ (+3.59)} & \makecell{81.96 \\ (-0.75)} & \makecell{80.33 \\ (+3.43)} & \makecell{74.28 \\ (+3.50)} & \makecell{71.87 \\ (+3.09)} & \makecell{67.79 \\ (+2.34)} \\
 MetaMath-Mistral-7B & 43.63 & 75.69 & 77.56 & 72.80 & 66.75 & 60.89 & 58.71 \\
\rowcolor{gray!25}
 + SFT on D & \makecell{49.72 \\ (+6.09)} & \makecell{82.33 \\ (+6.64)} & \makecell{78.24 \\ (+0.68)} & \makecell{77.32 \\ (+4.52)} & \makecell{71.13 \\ (+4.38)} & \makecell{68.78 \\ (+7.89)} & \makecell{64.42 \\ (+5.71)} \\
 \midrule
 \multicolumn{8}{c}{Other 7B Models} \\
 \midrule
 llemma\_7b & 2.06 & 66.63 & 28.81 & 27.64 & 23.10 & 20.05 & 19.19 \\
\rowcolor{gray!25}
 + SFT on D & \makecell{33.05 \\ (+30.99)} & \makecell{80.71 \\ (+14.08)} & \makecell{67.17 \\ (+38.36)} & \makecell{62.59 \\ (+34.95)} & \makecell{58.09 \\ (+34.99)} & \makecell{54.54 \\ (+34.49)} & \makecell{54.21 \\ (+35.02)} \\
 deepseek-math-7b & 42.98 & 69.07 & 81.88 & 76.57 & 66.67 & 62.79 & 56.55 \\
\rowcolor{gray!25}
 + SFT on D & \makecell{51.31 \\ (+8.33)} & \makecell{80.34 \\ (+11.27)} & \makecell{81.35 \\ (-0.53)} & \makecell{77.91 \\ (+1.34)} & \makecell{72.35 \\ (+5.68)} & \makecell{67.88 \\ (+5.09)} & \makecell{65.36 \\ (+8.81)} \\
MetaMath-Llemma-7B & 28.18 & 64.77 & 68.23 & 62.34 & 53.81 & 49.55 & 44.19 \\
\rowcolor{gray!25}
 + SFT on D & \makecell{38.86 \\ (+10.68)} & \makecell{77.32 \\ (+12.55)} & \makecell{70.96 \\ (+2.73)} & \makecell{67.78 \\ (+5.44)} & \makecell{62.73 \\ (+8.92)} & \makecell{57.62 \\ (+8.07)} & \makecell{54.87 \\ (+10.68)} \\
 \midrule
 \multicolumn{8}{c}{LLaMA-2-13B Models} \\
 \midrule
LLaMA-2-13B & 8.61 & 70.18 & 37.76 & 36.32 & 29.83 & 27.95 & 26.50 \\
\rowcolor{gray!25}
 + SFT on D & \makecell{37.27 \\ (+28.66)} & \makecell{84.78 \\ (+14.60)} & \makecell{66.49 \\ (+28.73)} & \makecell{66.03 \\ (+29.71)} & \makecell{61.42 \\ (+31.59)} & \makecell{58.62 \\ (+30.67)} & \makecell{56.37 \\ (+29.87)} \\
 MAmmoTH-13B & 18.63 & 74.07 & 55.12 & 52.97 & 45.76 & 45.01 & 40.82 \\
\rowcolor{gray!25}
 + SFT on D & \makecell{42.32 \\ (+23.69)} & \makecell{85.54 \\ (+11.47)} & \makecell{71.04 \\ (+15.92)} & \makecell{69.12 \\ (+16.15)} & \makecell{65.62 \\ (+19.86)} & \makecell{62.25 \\ (+17.24)} & \makecell{60.77 \\ (+19.95)} \\
 WizardMath-13B & 19.29 & 72.12 & 57.77 & 54.90 & 45.49 & 42.29 & 41.67 \\
\rowcolor{gray!25}
 + SFT on D & \makecell{41.76 \\ (+22.47)} & \makecell{84.29 \\ (+12.17)} & \makecell{71.65 \\ (+13.88)} & \makecell{69.71 \\ (+14.81)} & \makecell{63.87 \\ (+18.38)} & \makecell{59.98 \\ (+17.69)} & \makecell{60.39 \\ (+18.72)} \\
 MetaMath-13B & 36.14 & 75.68 & 71.27 & 68.20 & 60.45 & 55.99 & 53.93 \\
\rowcolor{gray!25}
 + SFT on D & \makecell{44.10 \\ (+7.96)} & \makecell{79.38 \\ (+3.70)} & \makecell{73.84 \\ (+2.57)} & \makecell{71.38 \\ (+3.18)} & \makecell{65.97 \\ (+5.52)} & \makecell{63.07 \\ (+7.08)} & \makecell{58.61 \\ (+4.68)} \\
 \midrule
 \multicolumn{8}{c}{LLaMA-2-70B Models} \\
 \midrule
 LLaMA-2-70B & 26.50 & 81.19 & 59.74 & 57.82 & 51.18 & 49.55 & 48.50 \\
\rowcolor{gray!25}
 + SFT on D & \makecell{49.81 \\ (+23.31)} & \makecell{84.57 \\ (+3.38)} & \makecell{78.17 \\ (+18.43)} & \makecell{76.23 \\ (+18.41)} & \makecell{71.30 \\ (+20.12)} & \makecell{67.15 \\ (+17.60)} & \makecell{66.10 \\ (+17.60)} \\
 WizardMath-70B & 45.97 & 78.75 & 80.14 & 76.49 & 69.29 & 65.34 & 63.11 \\
\rowcolor{gray!25}
 + SFT on D & \makecell{54.68 \\ (+8.71)} & \makecell{82.60 \\ (+3.85)} & \makecell{82.41 \\ (+2.27)} & \makecell{80.59 \\ (+4.10)} & \makecell{74.89 \\ (+5.60)} & \makecell{71.87 \\ (+6.53)} & \makecell{68.07 \\ (+4.96)} \\
 MAmmoTH-70B & 42.98 & 85.24 & 72.93 & 74.48 & 69.20 & 64.52 & 62.17 \\
\rowcolor{gray!25}
 + SFT on D & \makecell{55.15 \\ (+12.17)} & \makecell{83.25 \\ (-1.99)} & \makecell{81.88 \\ (+8.95)} & \makecell{80.67 \\ (+6.19)} & \makecell{74.37 \\ (+5.17)} & \makecell{71.05 \\ (+6.53)} & \makecell{68.16 \\ (+5.99)} \\
 MetaMath-70B & 52.81 & 80.86 & 82.34 & 77.57 & 71.92 & 67.79 & 66.57 \\
\rowcolor{gray!25}
 + SFT on D & \makecell{57.12 \\ (+4.31)} & \makecell{84.55 \\ (+3.69)} & \makecell{83.17 \\ (+0.83)} & \makecell{80.92 \\ (+3.35)} & \makecell{75.59 \\ (+3.67)} & \makecell{72.05 \\ (+4.26)} & \makecell{70.32 \\ (+3.75)} \\
\bottomrule
\end{tabular}
\caption{Complete results of the effect of SFT on {\property}. 
All figures are in $\%$, and the SFT results are shaded. 
Differences between SFT results and original ones are shown in parentheses.}
\label{tabapp: sft_full_results}
\end{table*}

\subsection{Scaling up SFT Data}\label{app: scaleup}

 During the construction of the {\benchmark} (refer to Section~\ref{sec: dataset creation}), we use a round-by-round extension strategy, which can also be applied to augment the original GSM8K training set.
 The primary findings utilize $D = D_0 \cup D_1$ for SFT, and we can study the effect of enlarging our {\sftdata} through this specific extension strategy based on $D_1$.
 Consequently, we examine the effects of SFT on {\property} under four distinct scenarios: without SFT, SFT on $D_0$, SFT on $D_0, D_1$, SFT on $D_0, D_1, D_2$.
 Figure~\ref{fig: scaleup-e} and \ref{fig: scaleup-acc} have shown the performance in different settings, and the additional outcomes are presented in Figure~\ref{fig: scaleup-r} and \ref{fig: scaleup-acc-left}.

\begin{figure}
    \centering
    \includegraphics[width=1\linewidth]{Figures/scaleup-r.pdf}
    \caption{{\metricr} of scaling up {\sftdata} across various model scales in the LLaMA-2 family. }
    \label{fig: scaleup-r}
\end{figure}

\begin{figure*}
    \centering
    \includegraphics[width=1\linewidth]{Figures/scaleup-acc-left.pdf}
    \caption{The changes in $\text{Acc}_i$ when LLMs are fine-tuned on different {\sftdata} dataset. 
    Left: LLaMA-2-13B; right: LLaMA-2-70B.}
    \label{fig: scaleup-acc-left}
\end{figure*}

\newgeometry{top=0.05cm,bottom=0.1cm}
\begin{table*}[ht]
\centering
\footnotesize
\begin{tabular}{ccc|ccccc}
\toprule
\thead{Large Language Models} & \thead{CoLeG-E} & \thead{CoLeG-R} & \thead{$\text{Acc}_0$} & \thead{$\text{Acc}_1$} & \thead{$\text{Acc}_2$} & \thead{$\text{Acc}_3$} & \thead{$\text{Acc}_4$} \\
\midrule
\multicolumn{8}{c}{claude-3-haiku-20240307} \\
\midrule
Plan-and-Solve & 62.27 & 84.90 & 88.78 & 84.94 & 78.74 & 77.40 & 75.37 \\
\rowcolor{gray!25} + Prompt & \makecell{62.64 \\ (+0.37)} & \makecell{83.55 \\ (-1.35)} & \makecell{89.54 \\ (+0.76)} & \makecell{85.36 \\ (+0.42)} & \makecell{78.74 \\ (+0.00)} & \makecell{78.49 \\ (+1.09)} & \makecell{74.81 \\ (-0.56)} \\
Plan-and-Solve+ & 62.64 & 82.58 & 90.14 & 86.19 & 81.10 & 78.58 & 74.44 \\
\rowcolor{gray!25} + Prompt & \makecell{62.55 \\ (-0.09)} & \makecell{83.59 \\ (+1.01)} & \makecell{89.61 \\ (-0.53)} & \makecell{84.85 \\ (-1.34)} & \makecell{80.66 \\ (-0.44)} & \makecell{77.04 \\ (-1.54)} & \makecell{74.91 \\ (+0.47)} \\
Zero-Shot CoT & 62.83 & 83.07 & 89.61 & 85.52 & 80.05 & 77.13 & 74.44 \\
\rowcolor{gray!25} + Prompt & \makecell{64.14 \\ (+1.31)} & \makecell{83.56 \\ (+0.49)} & \makecell{89.31 \\ (-0.30)} & \makecell{86.69 \\ (+1.17)} & \makecell{81.36 \\ (+1.31)} & \makecell{77.22 \\ (+0.09)} & \makecell{74.63 \\ (+0.19)} \\
\midrule
\multicolumn{8}{c}{claude-3-opus-20240229} \\
\midrule
Plan-and-Solve & 74.81 & 84.07 & 95.45 & 92.30 & 88.28 & 85.30 & 80.24 \\
\rowcolor{gray!25} + Prompt & \makecell{78.00 \\ (+3.18)} & \makecell{87.07 \\ (+3.00)} & \makecell{95.60 \\ (+0.15)} & \makecell{92.47 \\ (+0.17)} & \makecell{88.89 \\ (+0.61)} & \makecell{86.12 \\ (+0.82)} & \makecell{83.24 \\ (+3.00)} \\
Plan-and-Solve+ & 75.00 & 84.79 & 95.30 & 91.38 & 87.49 & 84.48 & 80.81 \\
\rowcolor{gray!25} + Prompt & \makecell{78.28 \\ (+3.28)} & \makecell{86.01 \\ (+1.22)} & \makecell{95.91 \\ (+0.61)} & \makecell{92.72 \\ (+1.34)} & \makecell{88.54 \\ (+1.05)} & \makecell{86.03 \\ (+1.54)} & \makecell{82.49 \\ (+1.69)} \\
Zero-Shot CoT & 74.72 & 86.08 & 94.09 & 91.80 & 87.58 & 84.57 & 80.99 \\
\rowcolor{gray!25} + Prompt & \makecell{77.81 \\ (+3.09)} & \makecell{86.29 \\ (+0.21)} & \makecell{95.38 \\ (+1.29)} & \makecell{92.64 \\ (+0.84)} & \makecell{88.98 \\ (+1.40)} & \makecell{85.39 \\ (+0.82)} & \makecell{82.30 \\ (+1.31)} \\
\midrule
\multicolumn{8}{c}{gemini-pro} \\
\midrule
Plan-and-Solve & 46.25 & 77.35 & 80.74 & 75.82 & 69.99 & 65.15 & 62.45 \\
\rowcolor{gray!25} + Prompt & \makecell{47.10 \\ (+0.84)} & \makecell{79.48 \\ (+2.13)} & \makecell{80.82 \\ (+0.08)} & \makecell{76.57 \\ (+0.75)} & \makecell{71.48 \\ (+1.49)} & \makecell{65.34 \\ (+0.18)} & \makecell{64.23 \\ (+1.78)} \\
Plan-and-Solve+ & 48.22 & 79.19 & 80.52 & 76.82 & 70.25 & 66.88 & 63.76 \\
\rowcolor{gray!25} + Prompt & \makecell{49.91 \\ (+1.69)} & \makecell{81.99 \\ (+2.79)} & \makecell{80.74 \\ (+0.23)} & \makecell{78.33 \\ (+1.51)} & \makecell{71.57 \\ (+1.31)} & \makecell{66.88 \\ (+0.00)} & \makecell{66.20 \\ (+2.43)} \\
Zero-Shot CoT & 49.20 & 75.69 & 83.70 & 77.91 & 71.83 & 66.76 & 63.36 \\
\rowcolor{gray!25} + Prompt & \makecell{53.65 \\ (+4.45)} & \makecell{81.44 \\ (+5.75)} & \makecell{83.70 \\ (+0.00)} & \makecell{81.26 \\ (+3.35)} & \makecell{75.48 \\ (+3.65)} & \makecell{72.78 \\ (+6.02)} & \makecell{68.16 \\ (+4.81)} \\
\midrule
\multicolumn{8}{c}{glm-3-turbo} \\
\midrule
Plan-and-Solve & 42.03 & 75.58 & 81.79 & 74.79 & 71.30 & 65.76 & 61.82 \\
\rowcolor{gray!25} + Prompt & \makecell{39.94 \\ (-2.08)} & \makecell{77.33 \\ (+1.75)} & \makecell{82.04 \\ (+0.25)} & \makecell{77.66 \\ (+2.87)} & \makecell{71.80 \\ (+0.50)} & \makecell{67.06 \\ (+1.30)} & \makecell{63.44 \\ (+1.62)} \\
Plan-and-Solve+ & 44.09 & 80.66 & 81.41 & 75.21 & 71.37 & 68.40 & 65.67 \\
\rowcolor{gray!25} + Prompt & \makecell{42.79 \\ (-1.30)} & \makecell{78.59 \\ (-2.07)} & \makecell{82.57 \\ (+1.16)} & \makecell{78.11 \\ (+2.90)} & \makecell{70.95 \\ (-0.42)} & \makecell{67.39 \\ (-1.00)} & \makecell{64.89 \\ (-0.78)} \\
Zero-Shot CoT & 43.82 & 77.85 & 82.63 & 76.61 & 71.68 & 67.52 & 64.33 \\
\rowcolor{gray!25} + Prompt & \makecell{45.96 \\ (+2.14)} & \makecell{79.84 \\ (+1.99)} & \makecell{81.93 \\ (-0.70)} & \makecell{78.71 \\ (+2.10)} & \makecell{71.93 \\ (+0.25)} & \makecell{69.35 \\ (+1.83)} & \makecell{65.41 \\ (+1.09)} \\
\midrule
\multicolumn{8}{c}{gpt-3.5-turbo-0125} \\
\midrule
Plan-and-Solve & 41.76 & 80.43 & 78.70 & 76.65 & 70.87 & 67.15 & 63.30 \\
\rowcolor{gray!25} + Prompt & \makecell{42.98 \\ (+1.22)} & \makecell{81.86 \\ (+1.43)} & \makecell{79.38 \\ (+0.68)} & \makecell{78.24 \\ (+1.59)} & \makecell{71.39 \\ (+0.52)} & \makecell{67.60 \\ (+0.45)} & \makecell{64.98 \\ (+1.69)} \\
Plan-and-Solve+ & 48.03 & 81.14 & 80.67 & 78.83 & 72.70 & 68.87 & 65.45 \\
\rowcolor{gray!25} + Prompt & \makecell{50.09 \\ (+2.06)} & \makecell{81.12 \\ (-0.02)} & \makecell{81.96 \\ (+1.29)} & \makecell{78.58 \\ (-0.25)} & \makecell{73.49 \\ (+0.79)} & \makecell{71.05 \\ (+2.18)} & \makecell{66.48 \\ (+1.03)} \\
Zero-Shot CoT & 46.63 & 79.63 & 80.89 & 77.91 & 72.53 & 68.24 & 64.42 \\
\rowcolor{gray!25} + Prompt & \makecell{51.97 \\ (+5.34)} & \makecell{83.64 \\ (+4.01)} & \makecell{83.40 \\ (+2.50)} & \makecell{81.26 \\ (+3.35)} & \makecell{75.33 \\ (+2.80)} & \makecell{73.23 \\ (+4.99)} & \makecell{69.76 \\ (+5.34)} \\
\midrule
\multicolumn{8}{c}{gpt-3.5-turbo-instruct} \\
\midrule
Plan-and-Solve & 25.75 & 70.15 & 70.20 & 63.43 & 55.73 & 52.36 & 49.25 \\
\rowcolor{gray!25} + Prompt & \makecell{23.50 \\ (-2.25)} & \makecell{70.82 \\ (+0.67)} & \makecell{69.14 \\ (-1.06)} & \makecell{61.09 \\ (-2.34)} & \makecell{55.21 \\ (-0.52)} & \makecell{50.18 \\ (-2.18)} & \makecell{48.97 \\ (-0.28)} \\
Plan-and-Solve+ & 31.18 & 72.48 & 72.86 & 64.18 & 58.27 & 55.54 & 52.81 \\
\rowcolor{gray!25} + Prompt & \makecell{30.43 \\ (-0.75)} & \makecell{81.27 \\ (+8.78)} & \makecell{70.05 \\ (-2.81)} & \makecell{65.86 \\ (+1.67)} & \makecell{60.72 \\ (+2.45)} & \makecell{57.08 \\ (+1.54)} & \makecell{56.93 \\ (+4.12)} \\
Zero-Shot CoT & 31.84 & 71.90 & 74.75 & 69.79 & 61.33 & 57.71 & 53.75 \\
\rowcolor{gray!25} + Prompt & \makecell{35.96 \\ (+4.12)} & \makecell{80.17 \\ (+8.28)} & \makecell{73.69 \\ (-1.06)} & \makecell{68.20 \\ (-1.59)} & \makecell{62.64 \\ (+1.31)} & \makecell{60.34 \\ (+2.63)} & \makecell{59.08 \\ (+5.34)} \\
\midrule
\multicolumn{8}{c}{gpt-4-0125-preview} \\
\midrule
Plan-and-Solve & 75.66 & 86.12 & 94.92 & 92.47 & 87.23 & 83.85 & 81.74 \\
\rowcolor{gray!25} + Prompt & \makecell{75.47 \\ (-0.19)} & \makecell{84.29 \\ (-1.82)} & \makecell{95.53 \\ (+0.61)} & \makecell{92.55 \\ (+0.08)} & \makecell{86.96 \\ (-0.26)} & \makecell{84.21 \\ (+0.36)} & \makecell{80.52 \\ (-1.22)} \\
Plan-and-Solve+ & 75.84 & 84.79 & 95.30 & 92.22 & 86.70 & 84.21 & 80.81 \\
\rowcolor{gray!25} + Prompt & \makecell{76.03 \\ (+0.19)} & \makecell{85.19 \\ (+0.40)} & \makecell{95.07 \\ (-0.23)} & \makecell{92.72 \\ (+0.50)} & \makecell{88.36 \\ (+1.66)} & \makecell{84.12 \\ (-0.09)} & \makecell{80.99 \\ (+0.19)} \\
Zero-Shot CoT & 76.69 & 85.68 & 95.07 & 92.64 & 87.66 & 84.75 & 81.46 \\
\rowcolor{gray!25} + Prompt & \makecell{77.53 \\ (+0.84)} & \makecell{85.40 \\ (-0.29)} & \makecell{95.83 \\ (+0.76)} & \makecell{93.05 \\ (+0.42)} & \makecell{87.58 \\ (-0.09)} & \makecell{84.30 \\ (-0.45)} & \makecell{81.84 \\ (+0.37)} \\
\bottomrule
\end{tabular}
\caption{Complete results of various proprietary LLMs with prompting methods on {\benchmark}. All figures are in \%, and methods with our proposed prompt method are shaded.}
\label{tabapp: full_prompting_results}
\end{table*}
\restoregeometry

\begin{table*}[ht]
\centering
\footnotesize
\begin{tabular}{ccc|ccccc}
\toprule
\thead{Model} & \thead{CoLeG-E} & \thead{CoLeG-R} & \thead{\(\text{Acc}_0\)} & \thead{\(\text{Acc}_1\)} & \thead{\(\text{Acc}_2\)} & \thead{\(\text{Acc}_3\)} & \thead{\(\text{Acc}_4\)} \\
\midrule
LLaMA-2-7B & 4.31 & 66.71 & 27.37 & 23.93 & 22.83 & 18.97 & 18.26 \\
 + SFT on $D_0$ & \makecell{20.22 \\ (+15.91)} & \makecell{66.64 \\ (-0.07)} & \makecell{58.45 \\ (+31.08)} & \makecell{49.62 \\ (+25.69)} & \makecell{42.96 \\ (+20.13)} & \makecell{40.93 \\ (+22.96)} & \makecell{38.95 \\ (+20.69)} \\
 + SFT on $D_0, D_1$ & \makecell{28.09 \\ (+23.78)} & \makecell{80.97 \\ (+14.26)} & \makecell{59.44 \\ (+32.07)} & \makecell{57.57 \\ (+33.64)} & \makecell{50.92 \\ (+28.09)} & \makecell{49.46 \\ (+30.49)} & \makecell{48.13 \\ (+29.87)} \\
 + SFT on $D_0, D_1, D_2$& \makecell{\textbf{30.34} \\ (+26.03)} & \makecell{\textbf{83.83} \\ (+17.12)} & \makecell{\textbf{60.65} \\ (+33.28)} & \makecell{\textbf{58.91} \\ (+35.98)} & \makecell{\textbf{53.89} \\ (+31.06)} & \makecell{\textbf{50.91} \\ (+32.14)} & \makecell{\textbf{50.84} \\ (+32.18)} \\
\midrule
LLaMA-2-13B & 8.61 & 70.18 & 37.76 & 36.32 & 29.83 & 27.95 & 26.50 \\
 + SFT on $D_0$& \makecell{32.40 \\ (+23.79)} & \makecell{73.91 \\ (+3.73)} & \makecell{67.02 \\ (+29.26)} & \makecell{63.10 \\ (+26.78)} & \makecell{56.87 \\ (+27.04)} & \makecell{51.09 \\ (+23.14)} & \makecell{49.53 \\ (+23.03)} \\
 + SFT on $D_0, D_1$& \makecell{37.27 \\ (+28.66)} & \makecell{\textbf{84.78} \\ (+14.60)} & \makecell{66.49 \\ (+28.73)} & \makecell{66.03 \\ (+29.71)} & \makecell{61.42 \\ (+31.59)} & \makecell{58.62 \\ (+30.67)} & \makecell{\textbf{56.37} \\ (+29.87)} \\
 + SFT on $D_0, D_1, D_2$& \makecell{\textbf{38.86} \\ (+30.25)} & \makecell{80.05 \\ (+9.87)} & \makecell{\textbf{69.60} \\ (+31.84)} & \makecell{\textbf{70.63} \\ (+34.31)} & \makecell{\textbf{62.99} \\ (+33.16)} & \makecell{\textbf{59.44} \\ (+31.49)} & \makecell{55.71 \\ (+29.21)} \\
\midrule
LLaMA-2-70B & 26.50 & 81.19 & 59.74 & 57.82 & 51.18 & 49.55 & 48.50 \\
+ SFT on $D_0$& \makecell{45.32 \\ (+18.82)} & \makecell{81.76 \\ (+0.57)} & \makecell{76.27 \\ (+16.53)} & \makecell{74.90 \\ (+17.08)} & \makecell{69.12 \\ (+17.94)} & \makecell{66.42 \\ (+16.87)} & \makecell{62.36 \\ (+13.86)} \\
 + SFT on $D_0, D_1$& \makecell{49.81 \\ (+23.31)} & \makecell{\textbf{84.57} \\ (+3.38)} & \makecell{78.17 \\ (+18.43)} & \makecell{\textbf{76.23} \\ (+18.41)} & \makecell{71.30 \\ (+20.12)} & \makecell{67.15 \\ (+17.60)} & \makecell{\textbf{66.10} \\ (+17.60)} \\
 + SFT on $D_0, D_1, D_2$& \makecell{\textbf{50.66} \\ (+24.16)} & \makecell{83.37 \\ (+2.18)} & \makecell{\textbf{78.39} \\ (+18.65)} & \makecell{75.98 \\ (+18.16)} & \makecell{\textbf{71.74} \\ (+20.56)} & \makecell{\textbf{68.51} \\ (+18.96)} & \makecell{65.36 \\ (+16.86)} \\
\bottomrule
\end{tabular}
\caption{Complete results of the effect of scaling up {\sftdata} on {\property}. 
All figures are in $\%$.
Differences between the SFT results and the original are shown in parentheses.
The best results within each model scale are shown in bold.
In general, scaling up {\sftdata} can improve {\property}.}
\label{tabapp: scaleup_results}
\end{table*}
